# Supplementary material for: Big Bang Nucleosynthesis Limits and Relic Gravitational Waves Detection Prospects
Source: arXiv:2111.09541 source file (2022-06-18)
Supplement: Supplementary file 1 [file supplement_include.tex]

\setlength{\topmargin}{-14mm}
\usepackage{graphicx,bm,color,braket}
\graphicspath{{./fig/}{./png/}}

%|||||||||||||||||||||||||||||||||||||||||||||||||||||||||||||||||||
%             Customized Commands
%|||||||||||||||||||||||||||||||||||||||||||||||||||||||||||||||||||
%  mathematical abbreviations
%
%
%

%\newcommand{\BoldVec}[1]{\bm{#1}}}
%
% math debs
\newcommand{\EQ}{\begin{equation}}
\newcommand{\EN}{\end{equation}}
\newcommand{\EQA}{\begin{eqnarray}}
\newcommand{\ENA}{\end{eqnarray}}

%\newcommand{\Sec}[1]{\S\,\ref{#1}}
%\newcommand{\Secs}[2]{\S\S\,\ref{#1} and~\ref{#2}}

%\newcommand{\bra}[1]{\langle #1\rangle}

 %redundant

{}
{}
{}

%
% tilde
%

%
%  unit vectors
%

%
%  hatted quantities
%

%
%  vectors
%

 %(convert aaa -> aaaa, compatibility problem)

%
%  correlation tensors
%

%
%  operators  (roman)
%

%
%  numbers
%

%\def\kf{k_\ast}

%

%

%

%
%  journals
%

\usepackage{nicefrac}
